# Supplementary material for: Generic mobility edges in several classes of duality-breaking one-dimensional quasiperiodic potentials
Source: arXiv:2304.06081 source file (2023-06-29)

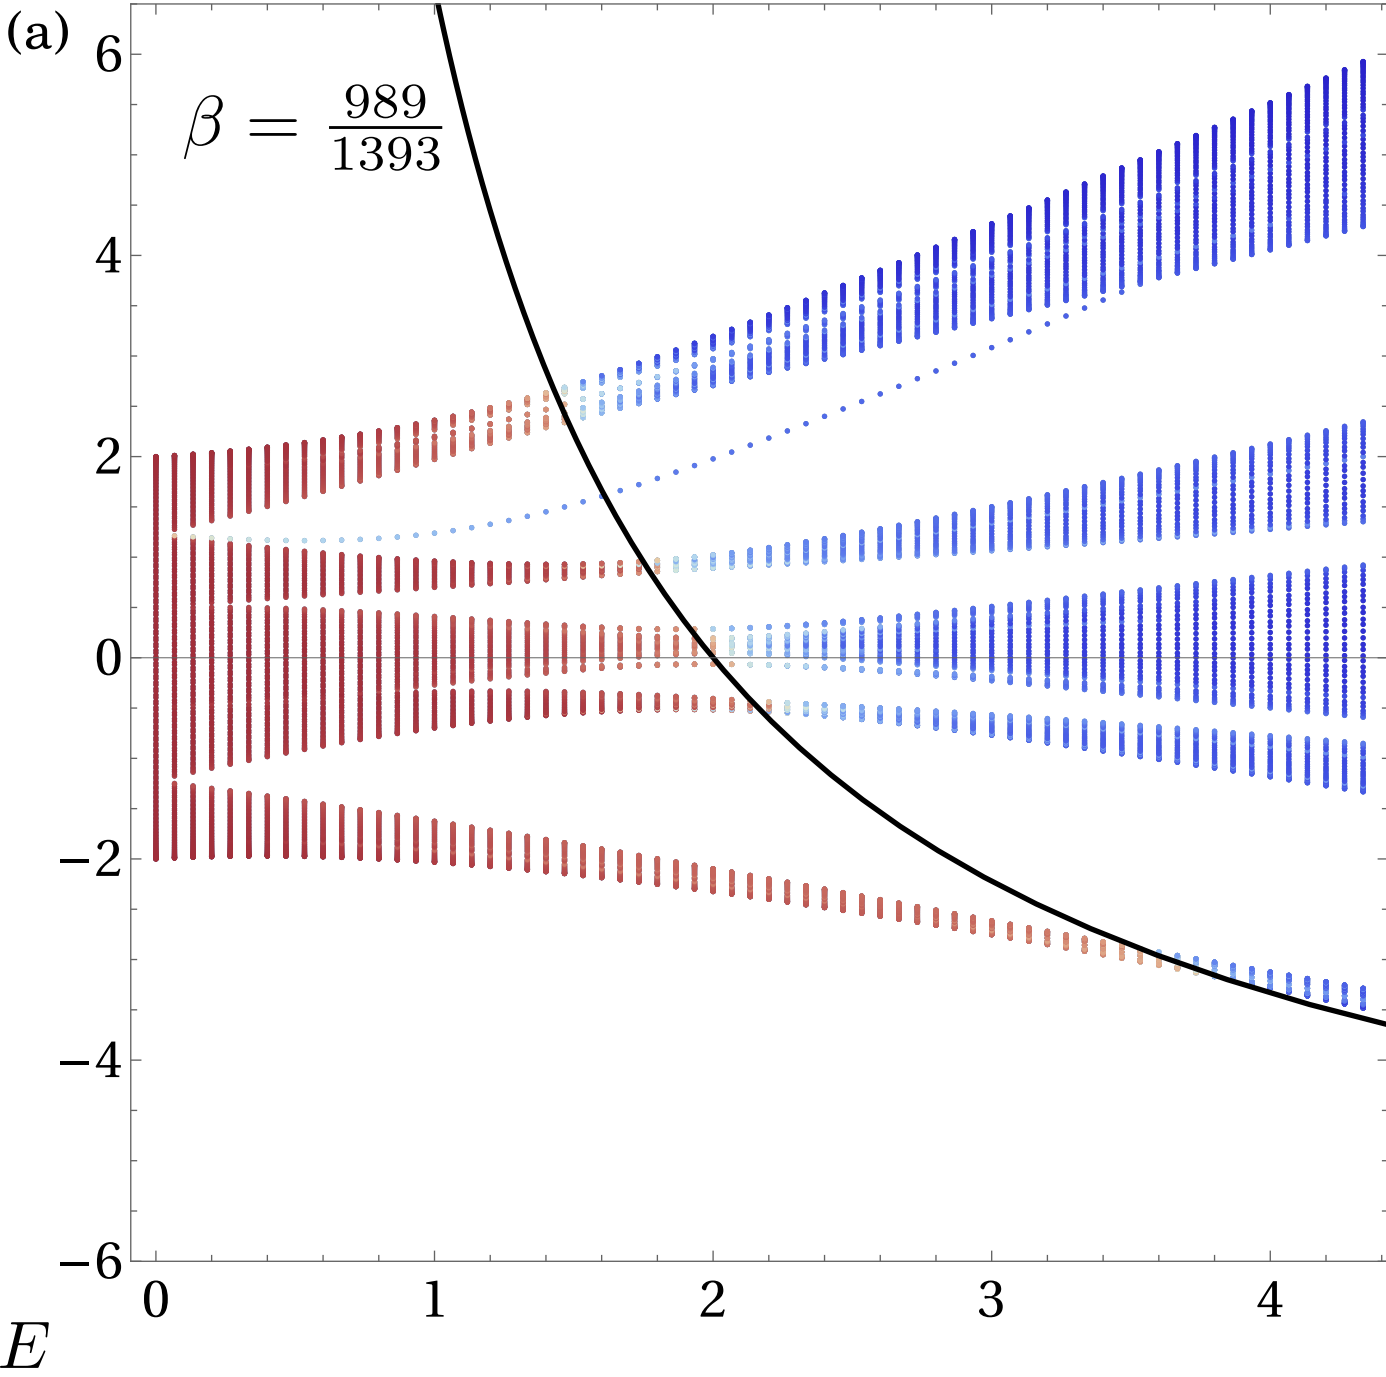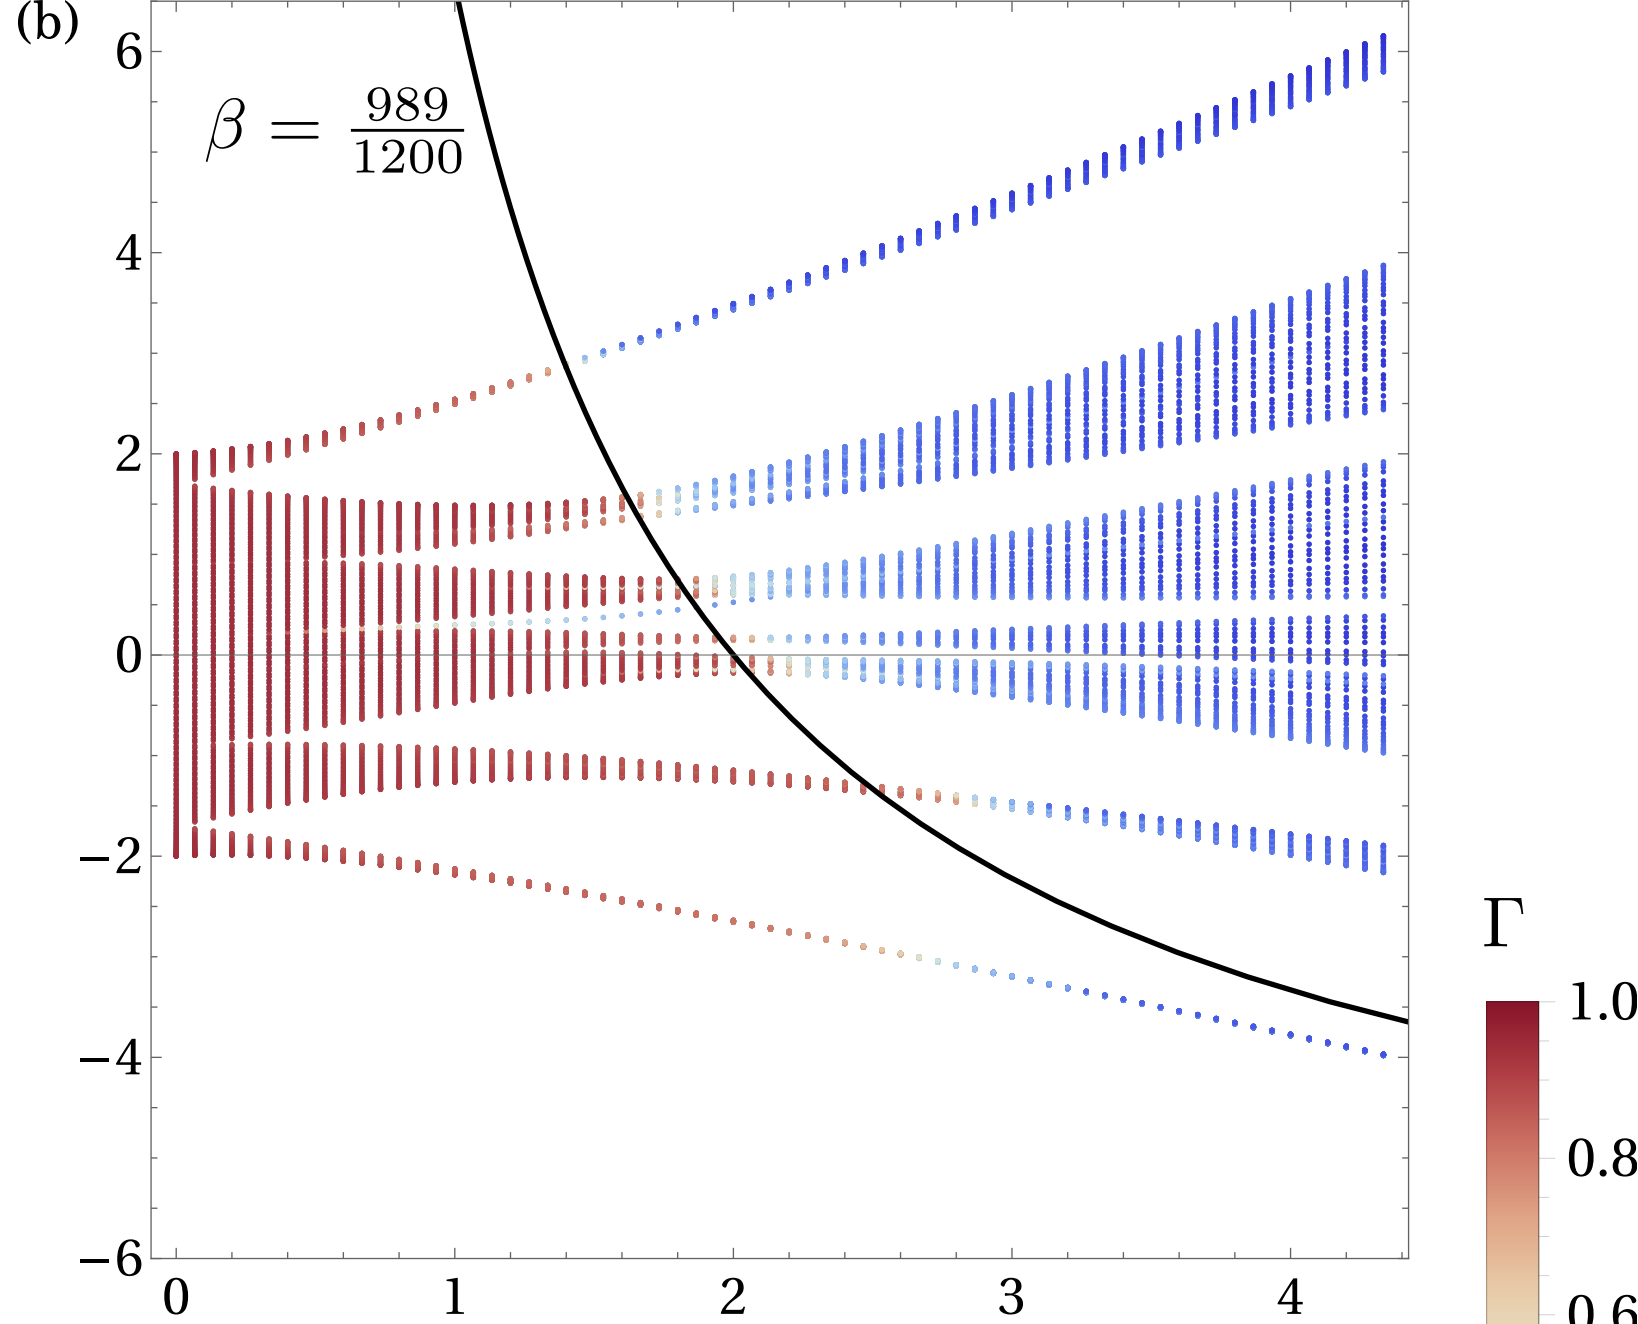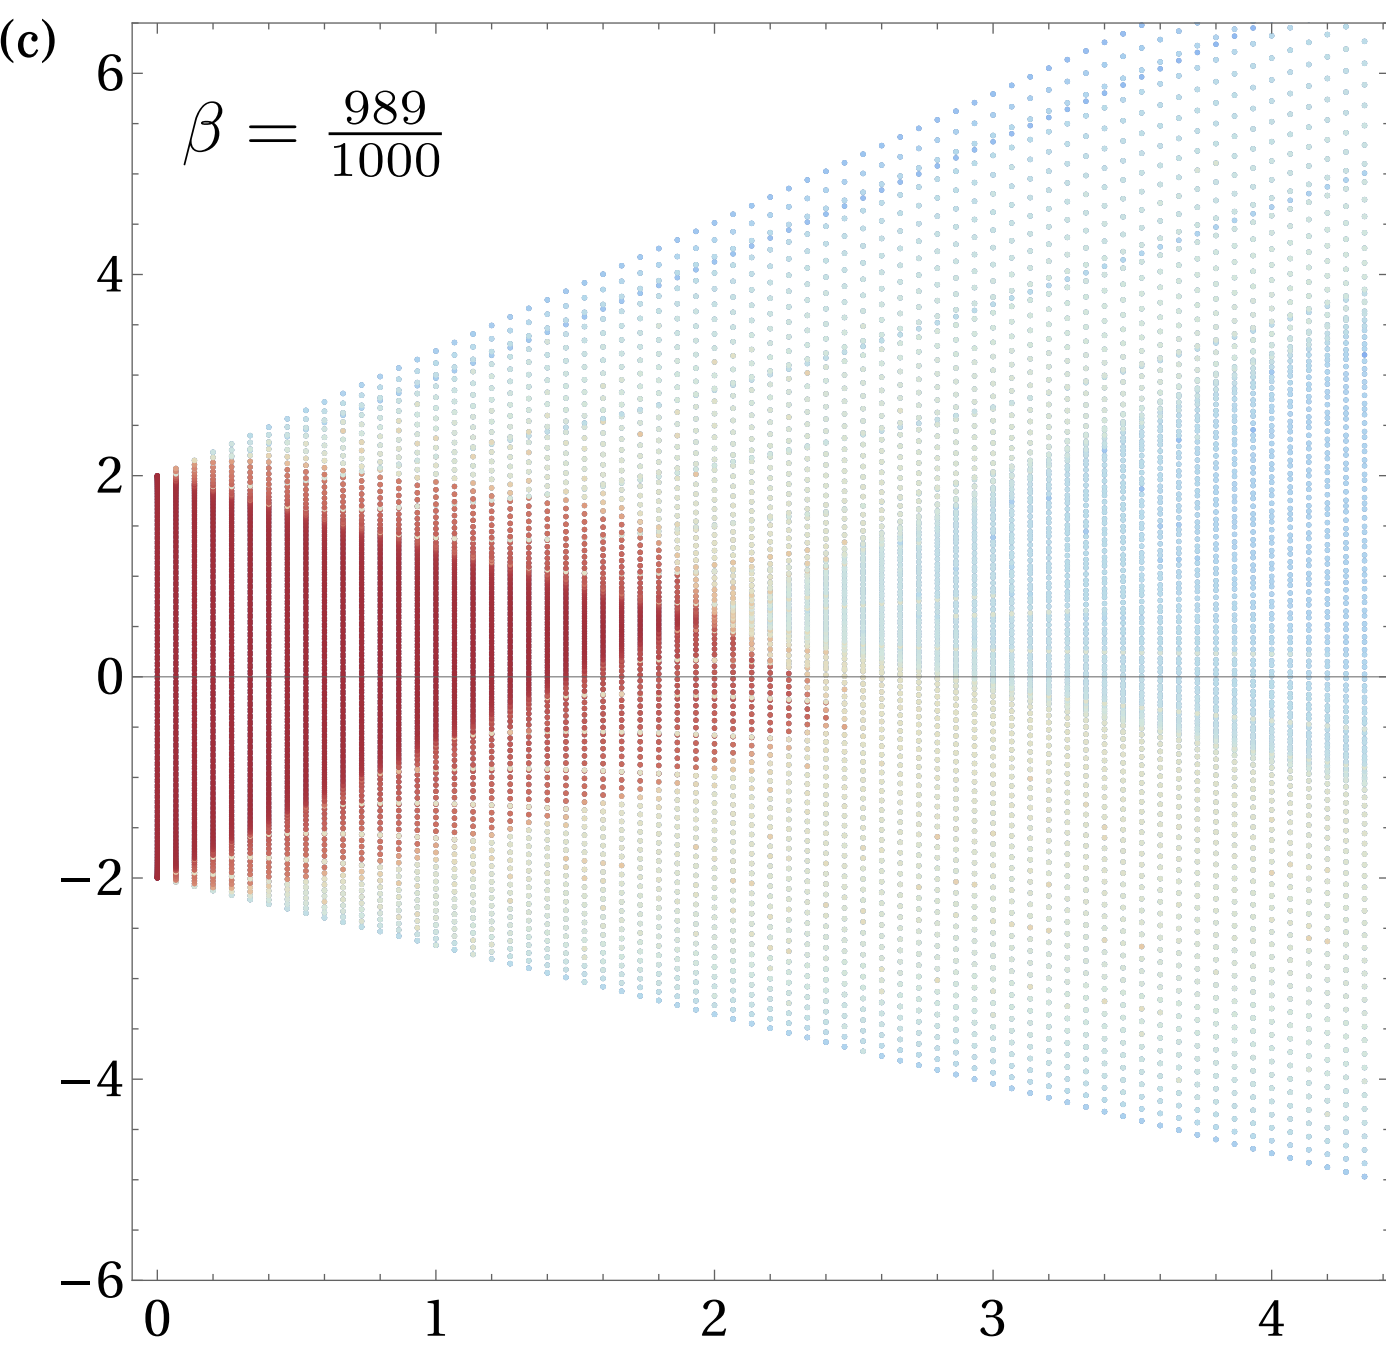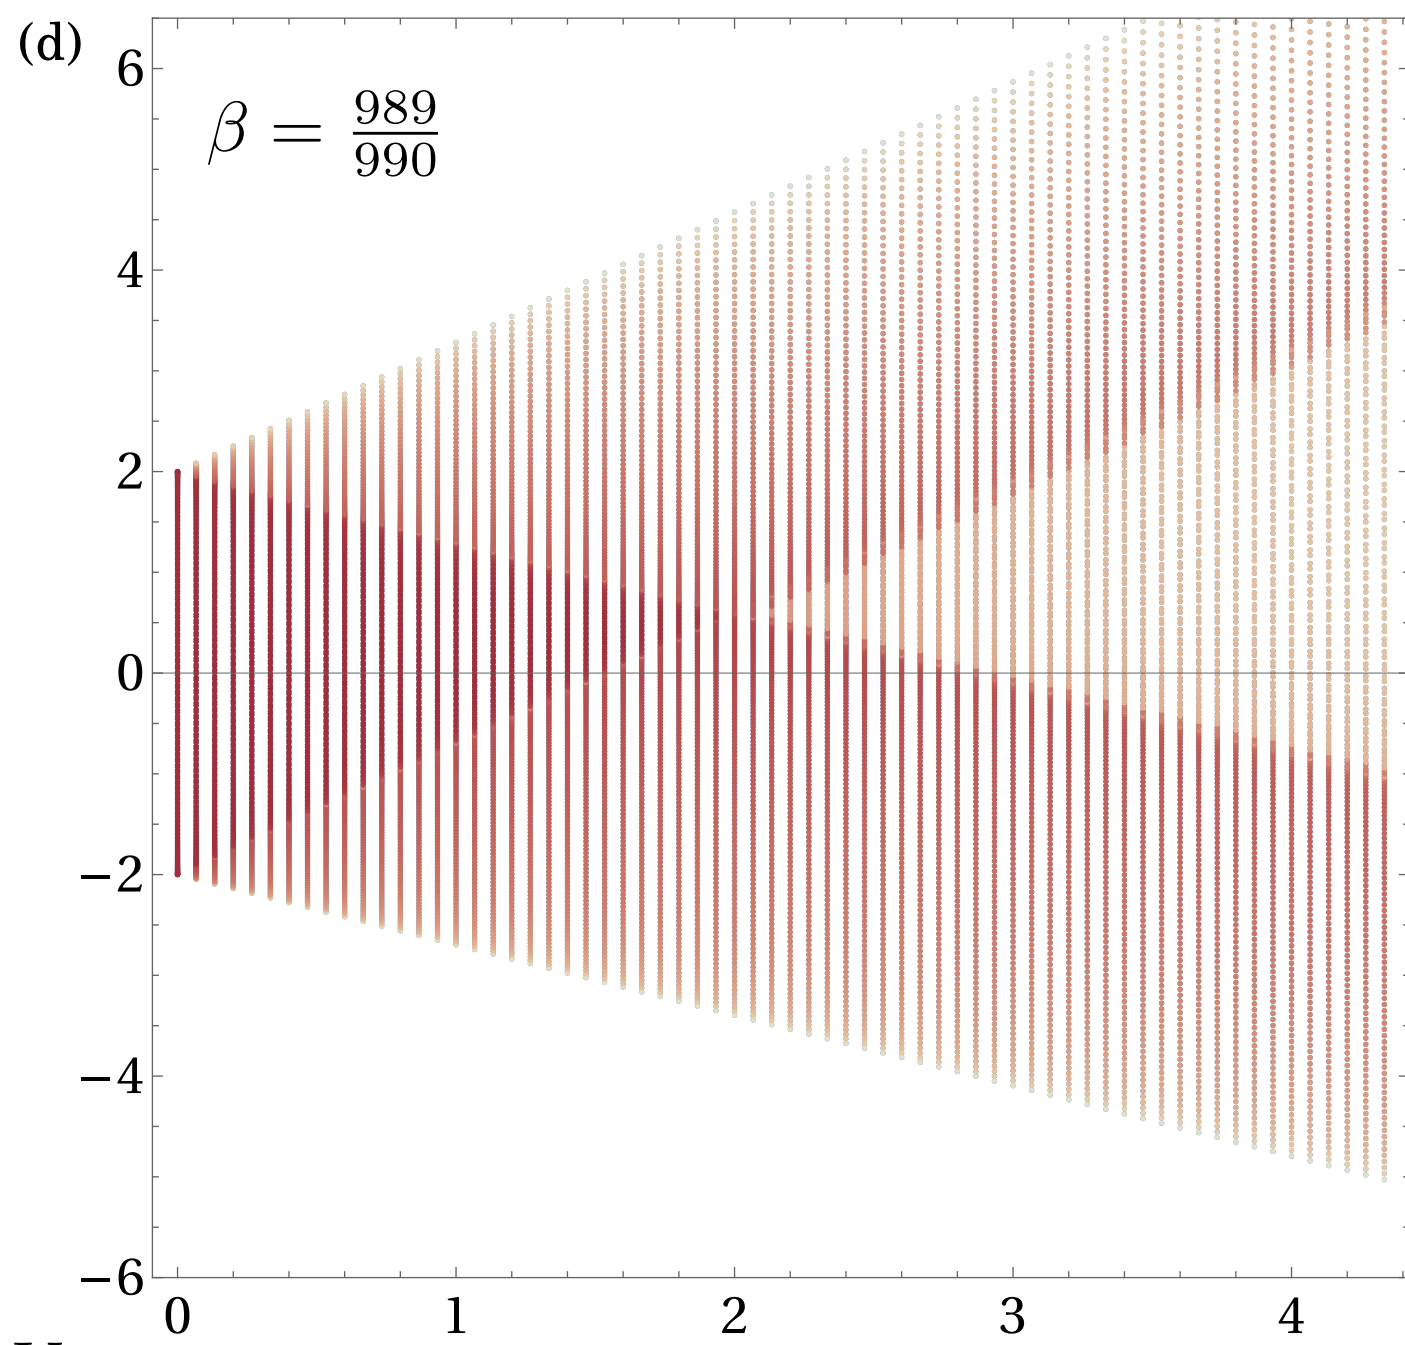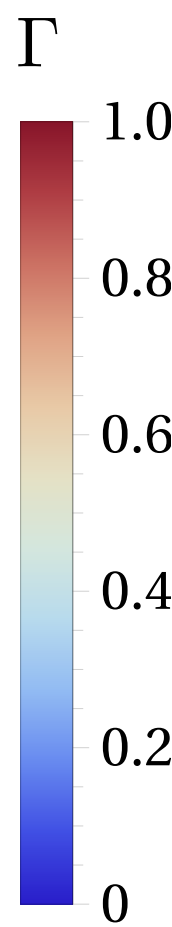

Supplement: Supplementary file 1 [file appendix.pdf]
